# Supplementary material for: MVDD: Multi-View Depth Diffusion Models
Source: arXiv:2312.04875 source file (2023-12-19)
Supplement: Supplementary file 1 [file appendix.tex]

\section{Content}
\label{sec:rationale}
The supplemental material is organized as follows:
\begin{itemize}
\item In~\cref{sec:metrics}, we introduce metrics used in the main paper;
\item In~\cref{sec:cam}, we introduce the detailed camera embeddings and setup;
\item In~\cref{sec:network}, we provide more details on the network architectures;
% \item In~\cref{sec:quan}, we report more quantitative results in addition to those in the main paper;
\item In~\cref{sec:quan}, we present more quantitative and qualitative results in addition to those in the main paper;
\item In~\cref{sec:codebase}, we list used codebases in this paper. 

\end{itemize}

\section{Metrics}
\label{sec:metrics}
In line with previous research, we employ Chamfer distance (CD) and earth mover’s distance (EMD) to quantify the similarity among point clouds. Specifically, their formal definitions are as follows, in accordance with established methods:
\begin{equation}
\begin{aligned}
\mathrm{CD}(X, Y) & =\sum_{x \in X} \min _{y \in Y}\|x-y\|_2^2+\sum_{y \in Y} \min _{x \in X}\|x-y\|_2^2, \\
\operatorname{EMD}(X, Y) & =\min _{\gamma: X \rightarrow Y} \sum_{x \in X}\|x-\gamma(x)\|_2.
\end{aligned}
\end{equation}
Given two point clouds, $X$ and $Y$, with an equal number of points and $\gamma$ representing a bijection between them. 
Consider $\mathcal{S}_g$ as the collection of generated point clouds and $\mathcal{S}_r$ as the reference set of point clouds, both having an equal cardinality with $|\mathcal{S}_r| = |\mathcal{S}_r|$.

\begin{figure*}[t]
  \centering
%   \fbox{\rule{0pt}{3in} \rule{0.9\linewidth}{0pt}}
  \includegraphics[width=0.65\linewidth]{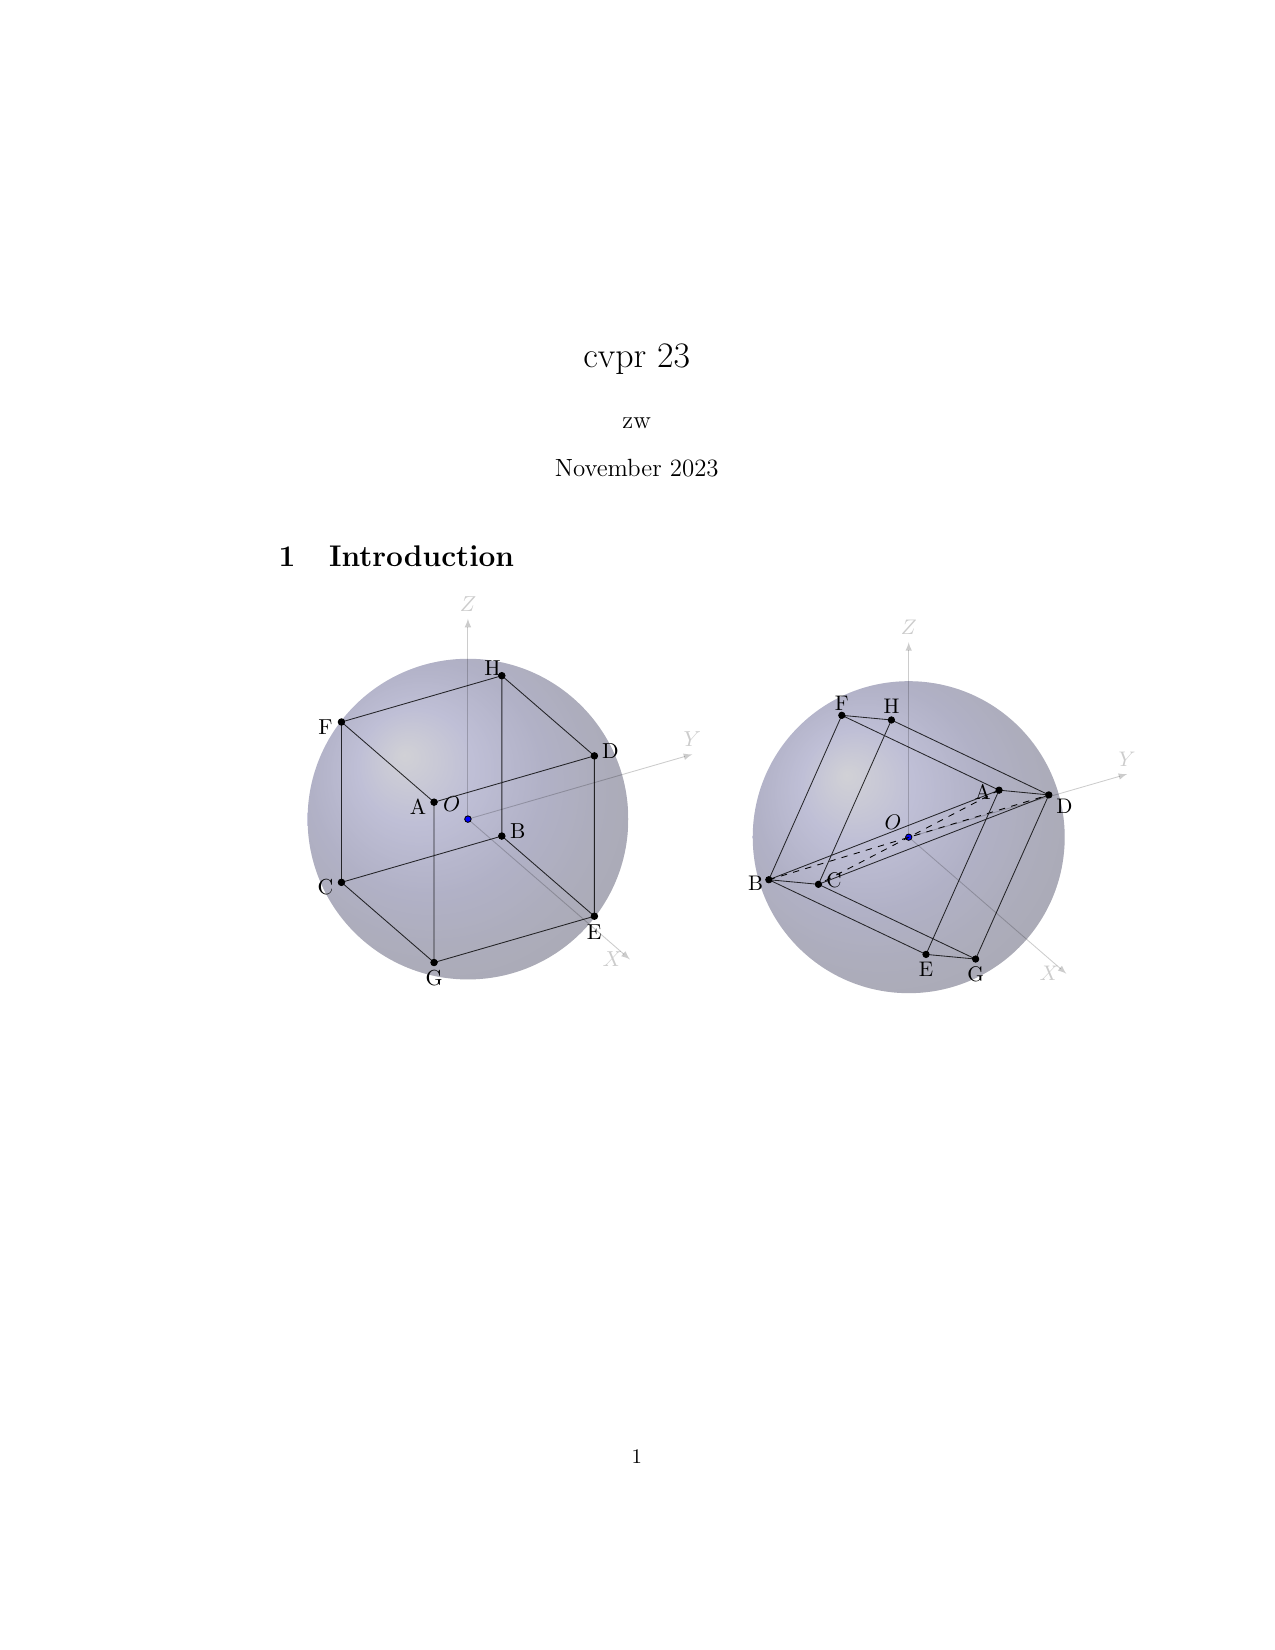}
    \captionsetup[sub]{font=normal,labelfont={bf,sf}}
    \hfill\subcaptionbox{\centering Fixed camera}[0.33\linewidth]
    \hfill\subcaptionbox{\centering Dynamic camera}[0.33\linewidth]
    % \hfill\subcaptionbox*{\centering Shape}[0.19\linewidth]
    % \hfill\subcaptionbox*{\centering  RGB}[0.19\linewidth]
    % \hfill\subcaptionbox*{\centering Depth}[0.19\linewidth]
    % \hfill\subcaptionbox*{\centering Shape}[0.19\linewidth]
    % \hfill\subcaptionbox{Airplane}[0.12\linewidth]
    
  \caption{Camera setup demonstration.}
  \label{fig:cam}
%   \vspace{-15pt}
\end{figure*}

Coverage (COV) calculates the proportion of point clouds within the reference set that find at least one corresponding match within the generated set. Every point cloud within the generated set is paired with its closest neighbor within the reference set, considering it a match.
\begin{equation}
\operatorname{COV}\left(\mathcal{S}_g, \mathcal{S}_r\right)=\frac{\left|\left\{\arg \min _{Y \in \mathcal{S}_r} D(X, Y) \mid X \in \mathcal{S}_g\right\}\right|}{\left|\mathcal{S}_r\right|}.
\end{equation}
When considering $D(\cdot, \cdot)$, which can be CD or EMD, it's important to note that while coverage can identify mode collapse, it does not assess the quality of generated point clouds. Surprisingly, it is feasible to attain a flawless coverage score even when the distances between generated and reference point clouds are excessively vast.

As a complementary to $\operatorname{COV}$, Minimum matching distance (MMD) involves calculating, for every point cloud within the reference set, the average distance to its closest neighbor in the generated set:
\begin{equation}
    \operatorname{MMD}\left(\mathcal{S}_g, \mathcal{S}_r\right)=\frac{1}{\left|\mathcal{S}_r\right|} \sum_{Y \in \mathcal{S}_r} \min _{X \in \mathcal{S}_g} D(X, Y),
\end{equation}
where $D(\cdot, \cdot)$ is chosen as either CD or EMD. The concept behind MMD involves computing the mean distance between point clouds within the reference set and their nearest counterparts in the generated set, thus serving as a metric to assess quality.

Lopez-Paz and Oquab~\cite{lopez2016revisiting} introduced this method for conducting two-sample tests, determining the similarity between two distributions. Additionally, it has been investigated as a metric for assessing GANs~\cite{xu2018empirical}. When considering $\mathcal{S}_{-X} = \mathcal{S}_r \cup \mathcal{S}_g - {X}$ and $N_X$ representing the nearest neighbor of $X$ in $\mathcal{S}_{-X}$, 1-NNA denotes the leave-one-out accuracy of the 1-nearest neighbor classifier.
\begin{equation}
\begin{aligned}
    1-\mathrm{NNA} & \left(\mathcal{S}_g, \mathcal{S}_r\right)   \\
    & = \frac{\sum_{X \in \mathcal{S}_g} \mathbb{I}\left[N_X \in \mathcal{S}_g\right] +\sum_{Y \in \mathcal{S}_r} \mathbb{I}\left[N_Y \in \mathcal{S}_r\right]}{\left|\mathcal{S}_g\right|+\left|\mathcal{S}_r\right|},
\end{aligned}
\end{equation}
where the function $\mathbb{I}[\cdot]$ is the indicator. With every instance, the 1-NN classifier distinguishes it as belonging to either $\mathcal{S}_r$ or $\mathcal{S}_g$, depending on the closest sample's label. If $\mathcal{S}_r$ and $\mathcal{S}_g$ are drawn from the same source, this classifier's accuracy should eventually stabilize at 50\% with a sufficient number of samples. The closer this accuracy gets to 50\%, the more similarity exists between $\mathcal{S}_g$ and $\mathcal{S}_r$, indicating the model's proficiency in modeling the target distribution. In our scenario, computing the nearest neighbor can be done using CD or EMD.  Unlike COV and MMD, 1-NNA directly gauges the similarity in distributions, considering both diversity and quality simultaneously.

\section{Cameras}
\label{sec:cam} 

\subsection{Camera embeddings}
In each step of the diffusion process, we also condition a set of extrinsic camera parameters $c \in \mathbb{R} ^{F \times 16}$ into the model.
According to~\cite{shi2023mvdream}, we found that embedding camera parameters with a 2-layer MLP leads to the most satisfying image quality with distinguishable
view differences and we also add camera embeddings to time embeddings as residuals.
\begin{equation}
\mathbf{z}=\text{MLP}\left(\operatorname{PosEnc}\left(\sqrt{\bar{\alpha}_t}\right)\right)+\text{MLP}(\operatorname{Embedding}(c)),
\end{equation}
where $\operatorname{PosEnc}$ is the sinusoidal positional encoding used
in Transformer~\cite{vaswani2017attention} as follows:
\begin{equation}
\begin{aligned}
& \operatorname{PosEnc}_{t, i}^{(1)}=\sin \left(\frac{t}{10000^{\frac{i}{d-1}}}\right), \\
& \operatorname{PosEnc}_{t, i}^{(2)}=\cos \left(\frac{t}{10000^{\frac{i}{d-1}}}\right).
\end{aligned}
\end{equation}
$\operatorname{Embedding}$ is the embedding
layer. We use adaptive group normalization layers (AdaGN) following ~\cite{dhariwal2021diffusion} to incorporate embedding vector $\mathbf{z}$  into every residual block. AdaGN realize 
group normalization through channel-wise scaling and
shifting w.r.t. normalized feature maps in each block of U-Net.
% \begin{equation}
%     \operatorname{AdaGN}(\mathbf{h}, \mathbf{z})=\mathbf{z}_s\left(\operatorname{GroupNorm}(\mathbf{h})+\mathbf{z}_t\right)
% \end{equation}

\subsection{Camera placement}
For shape generation task as we describe in Sec. 4.1 in the main paper, since we have the control over the location of the camera, we place the eight cameras on the eight vertices (A, B, C, D, E, F, G and H) of a cuboid as shown in~\cref{fig:cam}(a) to make sure it covers the whole object. All vertices are on a sphere of radius $r=\sqrt{3}$. Specifically, vertices A, F, H, D are placed with elevation angle $30^\circ$ and azimuth angle $45^\circ$, $135^\circ$, $225^\circ$ and $315^\circ$, respectively. Vertices G, C, B, E are placed with elevation angle $-10^\circ$ and azimuth angle $45^\circ$, $135^\circ$, $225^\circ$ and $315^\circ$, respectively.

For depth completion task as we describe in Sec. 4.2 in the main paper, as the input depth image might come with any random pose, therefore, we place the first camera (denoted as node $A$ in~\cref{fig:cam}(b)) in a random location on the sphere. After that, we want to uniquely obtain the locations of the remaining cameras assuming that all the cameras are on a cube. Denoting the coordinate of the first freely placed camera A as $(X, Y, Z)$, we assume that the plane $ABCD$ always coincides with the plane $x / X = z/ Z$. In this way, the coordinates of the remaining vertices can be obtained as: 
\begin{equation}
\begin{aligned}
    B &= \operatorname{Rot}\left(n_{ABCD}, 2\operatorname{arctan}(\sqrt{2})\right) \cdot A , \\
    C & = \operatorname{Rot}\left(n_{ABCD}, 2\operatorname{arctan}(\sqrt{2}) + 2\operatorname{arctan}(1 / \sqrt{2})\right) \cdot A, \\
    D & = \operatorname{Rot}\left(n_{ABCD}, 4\operatorname{arctan}(\sqrt{2}) + 2\operatorname{arctan}(1 / \sqrt{2})\right) \cdot A, \\
    E & = \frac{A + B}{2} + \frac{AB \times AD}{||AB \times AD||}\cdot \frac{||AB||}{2}, \\
    F & = \frac{A + B}{2} - \frac{AB \times AD}{||AB \times AD||}\cdot \frac{||AB||}{2}, \\
    G & = \frac{C + D}{2} + \frac{AB \times AD}{||AB \times AD||}\cdot \frac{||AB||}{2}, \\
    H & = \frac{C + D}{2} - \frac{AB \times AD}{||AB \times AD||}\cdot \frac{||AB||}{2}, \\
\end{aligned}   
\end{equation}
where $n_{ABCD}$ is the normal vector of the plane $ABCD$ and $\operatorname{Rot}(\cdot, \cdot)$ represents the rotation matrix with the first term as the axis to be rotated along and the second term as the angle to rotate along the axis. To be concrete, following Euler–Rodrigues formula~\cite{dai2015euler}, we have:
\begin{equation}
\resizebox{\hsize}{!}{$
\operatorname{Rot}(\operatorname{n}, \theta) = \left[\begin{array}{ccc}
a^2+b^2-c^2-d^2 & 2(b c-a d) & 2(b d+a c) \\
2(b c+a d) & a^2+c^2-b^2-d^2 & 2(c d-a b) \\
2(b d-a c) & 2(c d+a b) & a^2+d^2-b^2-c^2
\end{array}\right],$}
\end{equation}
where $a = \operatorname{cos}(\theta / 2)$, $b, c, d = -\frac{n}{||n||} \operatorname{sin}(\theta / 2)$.

\begin{table}[!t]
\centering
\resizebox{0.82\linewidth}{!}{

% \small
\centering
\setlength{\tabcolsep}{0.8em}
\begin{tabular}{lc}
\toprule
    Parameters & Values \\
\midrule
    Learning rate & $2e^{-4}$ \\
    Number of levels & $4$ \\
    U-Net base channels &  64 \\
    U-Net channel multiplier &  1, 2, 4, 8 \\
    U-Net residual block groups &  8 \\
    U-Net attention head &  4 \\
    U-Net attention head channels &  32 \\
    U-Net norm layer type &  GroupNorm \\
    % U-Net dropout & 0.0 & 0.0 & 0.0 & 0.1 & 0.1 & 0.1 \\ 
    Diffusion steps &  1000 \\
    Noise schedule &  Cosine \\
    Clip input range & $[-1, 1]$ \\
\bottomrule
\end{tabular}}
% \vspace{1mm}
\caption{Hyper-parameters for diffusion models.
}
\label{tab:diff}
\end{table}

\begin{table*}
\centering
 \resizebox{0.87\linewidth}{!}{
\begin{tabular}{ccccccccc}
\toprule &  & Vox-diff \cite{zhou20213d} & DPM~\cite{luo2021diffusion} & 3D-LDM~\cite{nam20223d} & IM-GAN~\cite{chen2019learning} & PVD~\cite{zhou20213d} & LION~\cite{vahdat2022lion} & MVDD (Ours) \\
\hline \multirow{3}{*}{ Airplane } 
& MMD (CD) & 1.322 & 1.300  & 4.000 & \, \, 0.800 \mycirc[gold] &1.300 & 1.100 & \, \, 0.900 \mycirc[silver] \\ 
 & $\mathrm{COV}(\mathrm{CD}) $ & 11.82& 37.95 & 46.20 & 47.90& 43.97 & \, \, 50.74 \mycirc[gold]  & \, \, 48.25 \mycirc[silver] \\
& 1-NNA (CD) & 99.75& 88.56  & 74.00 & 67.74&69.22 & \, \, 64.36 \mycirc[gold] & \, \, 66.75 \mycirc[silver] \\
%  & MMD (EMD) & 1.561 &0.990 &  3.520 & 0.980  & 1.000  & \, \, 0.920 \mycirc[gold] &  \, \, 0.920 \mycirc[gold] \\
%  & $\mathrm{COV}$ (EMD) & 25.43 &  40.40 & 42.60 & 52.07  & 49.33 & 48.27 & \, \, 53.00 \mycirc[gold]\\
%  & 1-NNA (EMD) & 98.13& 73.47 & 80.10& 64.04& 64.89&  63.49  & \, \, 62.50 \mycirc[gold] \\
 \hline \multirow{3}{*}{ Car } 
 & MMD (CD) & 5.646 & 1.200  &  -& 1.103& 1.200 & \, \, 1.100 \mycirc[silver] & \, \, 1.000 \mycirc[gold] \\
& $\mathrm{COV}(\mathrm{CD})$ & 6.530 & 30.84 & -& \, \, 48.60 \mycirc[gold] & 31.11  & 36.72 & \, \, 47.93 \mycirc[silver] \\
 & 1-NNA (CD) & 99.56 & 93.31  & -& \, \, 66.74 \mycirc[silver] & 80.81 & 72.95 & \, \, 65.15 \mycirc[gold]\\
%  & MMD (EMD) & 1.551 & 0.710 & -& 0.640  &0.820 &0.900 & \, \, 0.620 \mycirc[gold]\\
%  & $\mathrm{COV}$ (EMD) & 22.15& 36.05 & - & 47.27 &39.51 & 42.59 & \, \, 49.53 \mycirc[gold]\\
%  & 1-NNA (EMD) & 96.83 &  80.33 & - &  57.04 & 71.29 &65.70 & \, \, 56.80 \mycirc[gold]\\
\hline \multirow{3}{*}{ Chair } 
& MMD (CD) & 5.840 & 3.400 & 16.80& 3.700 & 4.100 & \, \, 2.826 \mycirc[gold]& \, \, 3.200 \mycirc[silver]\\
 & $\mathrm{COV}(\mathrm{CD})$ & 17.52 &  48.27 & 42.60 & 48.29 & \, \, 50.07 \mycirc[silver] & 47.42 & \, \, 50.52 \mycirc[gold]  \\
 & 1-NNA (CD) & 97.12 & 64.77 &  \, \, 58.90 \mycirc[silver] & 60.19 &62.70 & 60.34 & \, \, 57.90 \mycirc[gold] \\
%  & MMD (EMD) & 2.930 & 2.140 & 8.200 & 2.200 &2.330 & \, \, 1.720 \mycirc[gold] & 2.110 \\
%  & $\mathrm{COV}$ (EMD) & 21.75 & 46.17 &  42.20 & 49.51 &46.47 &  50.52 & \, \, 51.55 \mycirc[gold] \\
%  & 1-NNA (EMD) & 96.74 &  65.73 & 65.30 & 55.54& 56.14  &  57.31 & \, \, 54.51 \mycirc[gold] \\
\bottomrule
\end{tabular}}
\caption{Unconditional generation on ShapeNet categories. MMD (CD) is multiplied by $10^3$. $\mycirc[gold]$ represents the best result and $\mycirc[silver]$ represents the second-best result.}
\label{tab:uncon}
% $\mycirc[gold]$ represents the best result, $\mycirc[silver]$ represent the second-best result and $\mycirc[brown]$ represents the third-best result.}
% \vspace{-15pt}
\end{table*}

\section{Network Architectures}
\label{sec:network}
We summarize the parameters of diffusion model in~\cref{tab:diff}.
To build the encoder of the U-Net, we utilize downsampling residual blocks and it consists of various levels, each with a distinct number of channels: {64, 128, 256, 512}. The process begins with an input resolution of 128 and progressively reduces to 64, 32, 16, 8 through downsampling.
For the decoder, we employ upsampling residual blocks. The number of output channels for each level in the decoder is set to 512, 256, 128, 64. For activation of each layer, a SiLU (Sigmoid Linear Unit) is used after convolution layer. 
The input depth map  has a resolution of $128\times128$. 
We use cosine noise scheduling defined as follows~\cite{nichol2021improved}:
\begin{equation}
\bar{\alpha}_t=\frac{f(t)}{f(0)}, \quad f(t)=\cos \left(\frac{t / T+s}{1+s} \cdot \frac{\pi}{2}\right)^2
\end{equation}
The details of the inference process for unconditional generation and depth completion are summarized in~\cref{alg:generation} and~\cref{alg:dc}, respectively.

% \begin{algorithm}
% \caption{Algorithm 2 Sampling}\label{alg:cap}
% \begin{algorithmic}[1]
% \Require $n \geq 0$
% \Ensure $y = x^n$
% \State $y \gets 1$
% % \State $X \gets x$
% % \State $N \gets n$
% \While{$N \neq 0$}
% \If{$N$ is even}
%     \State $X \gets X \times X$
%     \State $N \gets \frac{N}{2}$  \Comment{This is a comment}
% \ElsIf{$N$ is odd}
%     \State $y \gets y \times X$
%     \State $N \gets N - 1$
% \EndIf
% \EndWhile
% \end{algorithmic}
% \end{algorithm}

% for $t=T, \ldots, 1$ do

% $\mathbf{x}_{t-1}=\frac{1}{\sqrt{\alpha_t}}\left(\mathbf{x}_t-\frac{1-\alpha_t}{\sqrt{1-\bar{\alpha}_t}} \boldsymbol{\epsilon}_\theta\left(\mathbf{x}_t, t\right)\right)+\sigma_t \mathbf{z}$
% end for
% return $\mathrm{x}_0$

\begin{algorithm}[t]
\caption{Sampling for unconditional generation (Sec. 4.1)}\label{alg:generation}
\begin{algorithmic}[1]
\Require Diffusion model $\boldsymbol{\epsilon}_\theta\left(\mathbf{x}_t, t\right)$, $\alpha_t$, $\beta_t$
% \Ensure $y = x^n$
\State $\mathbf{x}_T \sim \mathcal{N}(\mathbf{0}, \mathbf{I})$
% \State $X \gets x$
% \State $N \gets n$
\For{ $t=T, \ldots, 1$}
    \State $\mathbf{\epsilon} \sim \mathcal{N}(\mathbf{0}, \mathbf{I})$ if $t>1$, else $\mathbf{\epsilon}=\mathbf{0}$
    \State $\mathbf{x}_{t-1}=\frac{1}{\sqrt{\alpha_t}}\left(\mathbf{x}_t-\frac{1-\alpha_t}{\sqrt{1-\tilde{\alpha}_t}} \boldsymbol{\epsilon}_\theta\left(\mathbf{x}_t, t\right)\right)+\sqrt{\beta_t} \mathbf{\epsilon}$ 
% \While{$N \neq 0$}
% \If{$N$ is even}
%     \State $X \gets X \times X$
%     \State $N \gets \frac{N}{2}$  \Comment{This is a comment}
% \ElsIf{$N$ is odd}
%     \State $y \gets y \times X$
%     \State $N \gets N - 1$
% \EndIf
% \EndWhile
\EndFor
\State \Return $\mathbf{x}_0$
\end{algorithmic}
\end{algorithm}

\section{Additional Results}
\label{sec:quan}

% \section{Additional qualitative results}
% \label{sec:qua}
We demonstrate the generated point cloud in more angles in~\cref{fig:chair}, \cref{fig:car} and~\cref{fig:airplane}. More qualitative results can be found in the accompanying supplementary webpage {\color{Blue}{\texttt{index.html}}}. We provide more quantitative results in~\cref{tab:uncon} in addition to Tab. 1 in the main paper. 
The generated point cloud, derived from our depth maps, showcases robust 3D coherence and validates efficacy of our suggested attention mechanism focusing on epipolar "line segments" and the depth fusion module. Conversely, existing point cloud-based diffusion models such as those in~\cite{vahdat2022lion,zhou20213d,luo2021diffusion} are constrained by their capacity to generate only 2048 points. This limitation hampers their ability to accurately capture intricate details within 3D shapes.

\paragraph{Auto-regressive v.s. our simultaneous generation.} We also compare with the baseline where each view of depth map is generated sequentially, i.e. the first view is generated first, the second view is conditioned on the first view and then the third view is generated conditioned on the first two views etc. As the results show in~\cref{tab:ablation}, our simultaneous strategy yields better results on unconditional generation task in ShapeNet~\cite{chang2015shapenet} chair category.

\begin{algorithm}[t]
\caption{Sampling for conditional generation (Sec. 4.2)}\label{alg:dc}
\begin{algorithmic}[1]
\Require Diffusion model $\boldsymbol{\epsilon}_\theta\left(\mathbf{x}_t, t\right)$, $\alpha_t$, $\beta_t$,  input depth map $\mathbf{x}_{0}^{\mathrm{in}}$
% \Ensure $y = x^n$
\State $\mathbf{x}^{\mathrm{other}}_T \sim \mathcal{N}(\mathbf{0}, \mathbf{I})$
% \State $X \gets x$
% \State $N \gets n$
\For{ $t=T, \ldots, 1$}
    % \State $\mathbf{\epsilon} \sim \mathcal{N}(\mathbf{0}, \mathbf{I})$ if $t>1$, else $\mathbf{\epsilon}=\mathbf{0}$
    \State  $\mathbf{x}_{t-1}^{\mathrm{in}} ~~\sim \mathcal{N}\left(\sqrt{\bar{\alpha}_t} \mathbf{x}^\mathrm{in}_0,\left(1-\bar{\alpha}_t\right) \mathbf{I}\right)$
    \State $\hat{\mathbf{x}}_{t-1}^{\mathrm{other}} \sim \mathcal{N}(\sqrt{1-\beta_t} ~\mathcal{\mu}_{\theta}(\mathbf{x}^{r_1:r_\NumNeighbors}_t, t), \beta_t\mathbf{I})$ \Comment{First pass}
    \State $\mathbf{x}_{t-1}^{\mathrm{other}} \sim \mathcal{N}(\mathcal{\mu}_{\theta}( \hat{\mathbf{x}}_{t-1}^{\mathrm{other}}, \mathbf{x}^{in}_0, t), \beta_t\mathbf{I})$ \Comment{Second pass}
% \While{$N \neq 0$}
% \If{$N$ is even}
%     \State $X \gets X \times X$
%     \State $N \gets \frac{N}{2}$  \Comment{This is a comment}
% \ElsIf{$N$ is odd}
%     \State $y \gets y \times X$
%     \State $N \gets N - 1$
% \EndIf
% \EndWhile
\EndFor
\State \Return $\mathbf{x}^\mathrm{other}_0$
\end{algorithmic}
\end{algorithm}

% \begin{table*}[t]
% \centering
% \large
%  \resizebox{0.6\linewidth}{!}{
% \begin{tabular}{ccccccccc}
% \toprule & SoftFlow~\cite{kim2020softflow}  & PointFlow~\cite{yang2019pointflow} &DPF-Net~\cite{klokov2020discrete} & PVD~\cite{zhou20213d} & MVDD (Ours) \\
% \hline \multirow{1}{*}{ Airplane } & 0.4042 & 0.4030 & 0.5279 & 0.4415 & 0.7315 \\
%  \multirow{1}{*}{ Chair } & 2.786 & 2.707 & 2.763 & 3.211 & 3.010  \\
%  \multirow{1}{*}{Car} & 1.850 & 1.803 & 1.396 & 1.774 & 0.900  \\
% % & MMD (CD) & 1.322 & 1.300  & 4.000 & \, \, 0.800 &1.300 & 1.100 & 0.900 \\ 
% %  & $\mathrm{COV}(\mathrm{CD}) $ & 11.82& 37.95 & 46.20 & 47.90& 43.97 & \, \, 50.74 \mycirc[gold]  & \, \, 48.25 \mycirc[silver] \\
% % & 1-NNA (CD) & 99.75& 88.56  & 74.00 & 67.74&69.22 & \, \, 64.36 \mycirc[gold] & \, \, 66.75 \mycirc[silver] \\
% \bottomrule
% \end{tabular}}
% \caption{Depth completion comparison against baselines. CD is multiplied by $10^3$.}
% \label{tab:dc}
% % $\mycirc[gold]$ represents the best result, $\mycirc[silver]$ represent the second-best result and $\mycirc[brown]$ represents the third-best result.}
% \end{table*}

\begin{table}[h]
    % \vskip 0.05in
  \begin{center}
  \resizebox{0.61\linewidth}{!}{
  \begin{tabular}{lccc} 
    \toprule
    & \multicolumn{2}{c}{\centering 1NN-A} \\% & \multicolumn{2}{c}{\centering COV} & \multicolumn{2}{c}{\centering 1NN-A}\\
    \cmidrule(l){2-3} % \cmidrule(l){7-8} \cmidrule(l){9-10} 
      &  CD  & EMD \\ %& CD  & EMD  & CD  & EMD\\
    \midrule
    Auto-regressive  & 70.23 & 68.13 \\
    Simultaneous & 57.90 & 54.51\\
    \bottomrule
  \end{tabular}}
 \end{center} \vspace{-15pt}
  \caption{Auto-regressive generation v.s. our simultaneous generation on the ShapeNet~\cite{chang2015shapenet} chair category. }
   \label{tab:ablation}
   \vspace{-15pt}
\end{table}

\begin{figure*}[t]
  \centering
%   \fbox{\rule{0pt}{3in} \rule{0.9\linewidth}{0pt}}
  \includegraphics[width=0.8\linewidth]{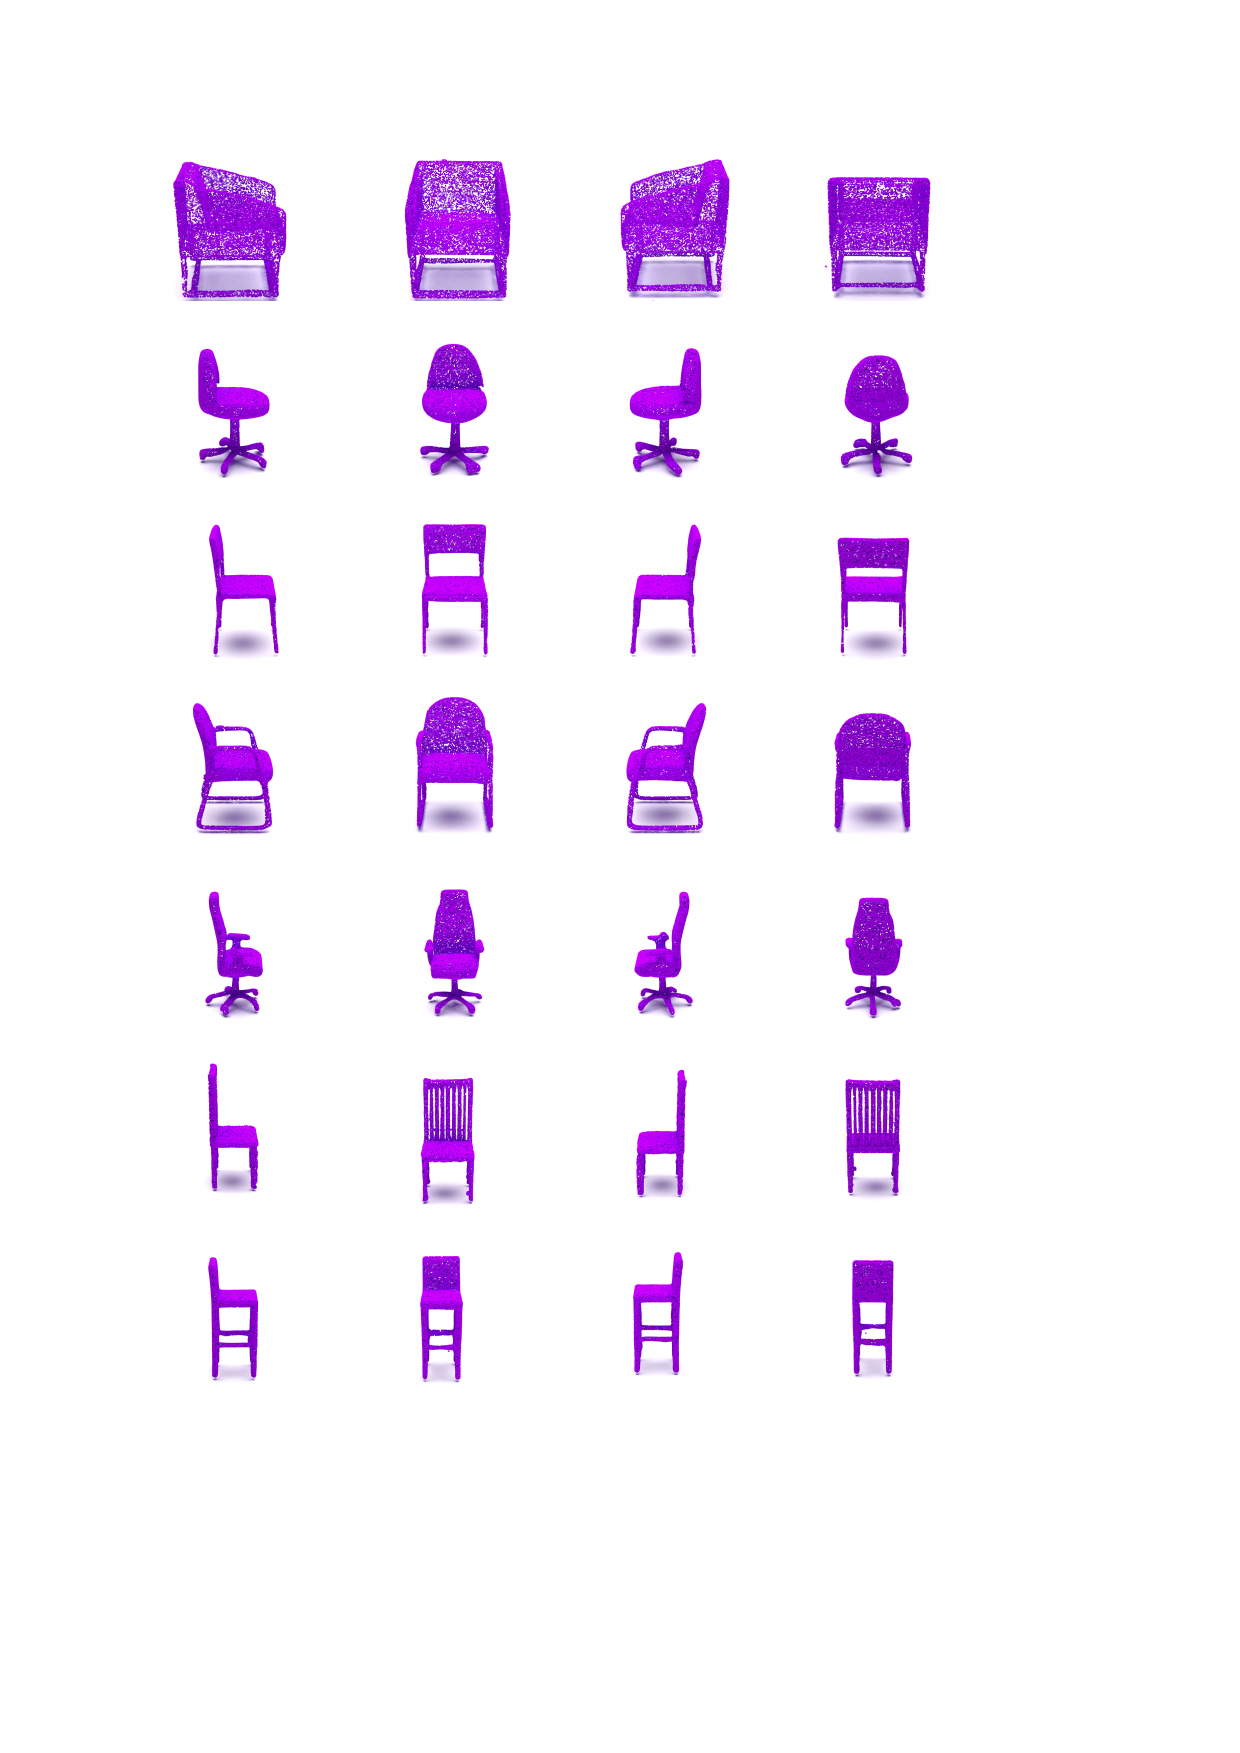}
    % \hfill\subcaptionbox*{\centering RGB}[0.19\linewidth]
    % \hfill\subcaptionbox*{\centering Depth}[0.19\linewidth]
    % \hfill\subcaptionbox*{\centering Shape}[0.19\linewidth]
    % \hfill\subcaptionbox*{\centering  RGB}[0.19\linewidth]
    % \hfill\subcaptionbox*{\centering Depth}[0.19\linewidth]
    % \hfill\subcaptionbox*{\centering Shape}[0.19\linewidth]
    % \hfill\subcaptionbox{Airplane}[0.12\linewidth]
    
  \caption{Generated chairs from more angles.}
  \label{fig:chair}
%   \vspace{90pt}
\end{figure*}

\section{Used codebases}
\label{sec:codebase}

Our diffusion model is based off of the github repo: \href{https://github.com/lucidrains/denoising-diffusion-pytorch}{https://github.com/lucidrains/denoising-diffusion-pytorch}.
The following codebases of the baselines are used: 
\begin{itemize}
    \item PVD~\cite{zhou20213d}: \href{https://github.com/alexzhou907/PVD}{https://github.com/alexzhou907/PVD} 
    \item LION~\cite{vahdat2022lion}: \href{https://github.com/nv-tlabs/LION}{https://github.com/nv-tlabs/LION}
    \item DPM~\cite{luo2021diffusion}: \href{https://github.com/luost26/diffusion-point-cloud}{https://github.com/luost26/diffusion-point-cloud}
\end{itemize}
We use other codebases for visualization and evaluation purposes:
\begin{itemize}
\item We use the MitSuba renderer for visualizations~\cite{nimier2019mitsuba}: \href{https://github.com/mitsuba-renderer/mitsuba3}{https://github.com/mitsuba-renderer/mitsuba3} and the code to generate the scene discription files for MitSuba: \href{https://github.com/zekunhao1995/PointFlowRenderer}{https://github.com/zekunhao1995/PointFlowRenderer}.
% (License: https://github.com/mitsuba-renderer/
% mitsuba2/blob/master/LICENSE), and the code to generate the scene discription files
% for MitSuba [31]: https://github.com/zekunhao1995/PointFlowRenderer.
\item We utilize SAP~\cite{peng2021shape} for mesh generation with the code at \href{https://github.com/
autonomousvision/shape\_as\_points}{https://github.com/
autonomousvision/shape\_as\_points}.
\item For calculating the evaluation metrics, we use the implementation for CD at \href{https:
//github.com/ThibaultGROUEIX/ChamferDistancePytorch}{https:
//github.com/ThibaultGROUEIX/ChamferDistancePytorch} and for
EMD at \href{https://github.com/daerduoCarey/PyTorchEMD}{https://github.com/daerduoCarey/PyTorchEMD}.
\end{itemize}

\begin{figure*}[t]
  \centering
%   \fbox{\rule{0pt}{3in} \rule{0.9\linewidth}{0pt}}
  \includegraphics[width=0.8\linewidth]{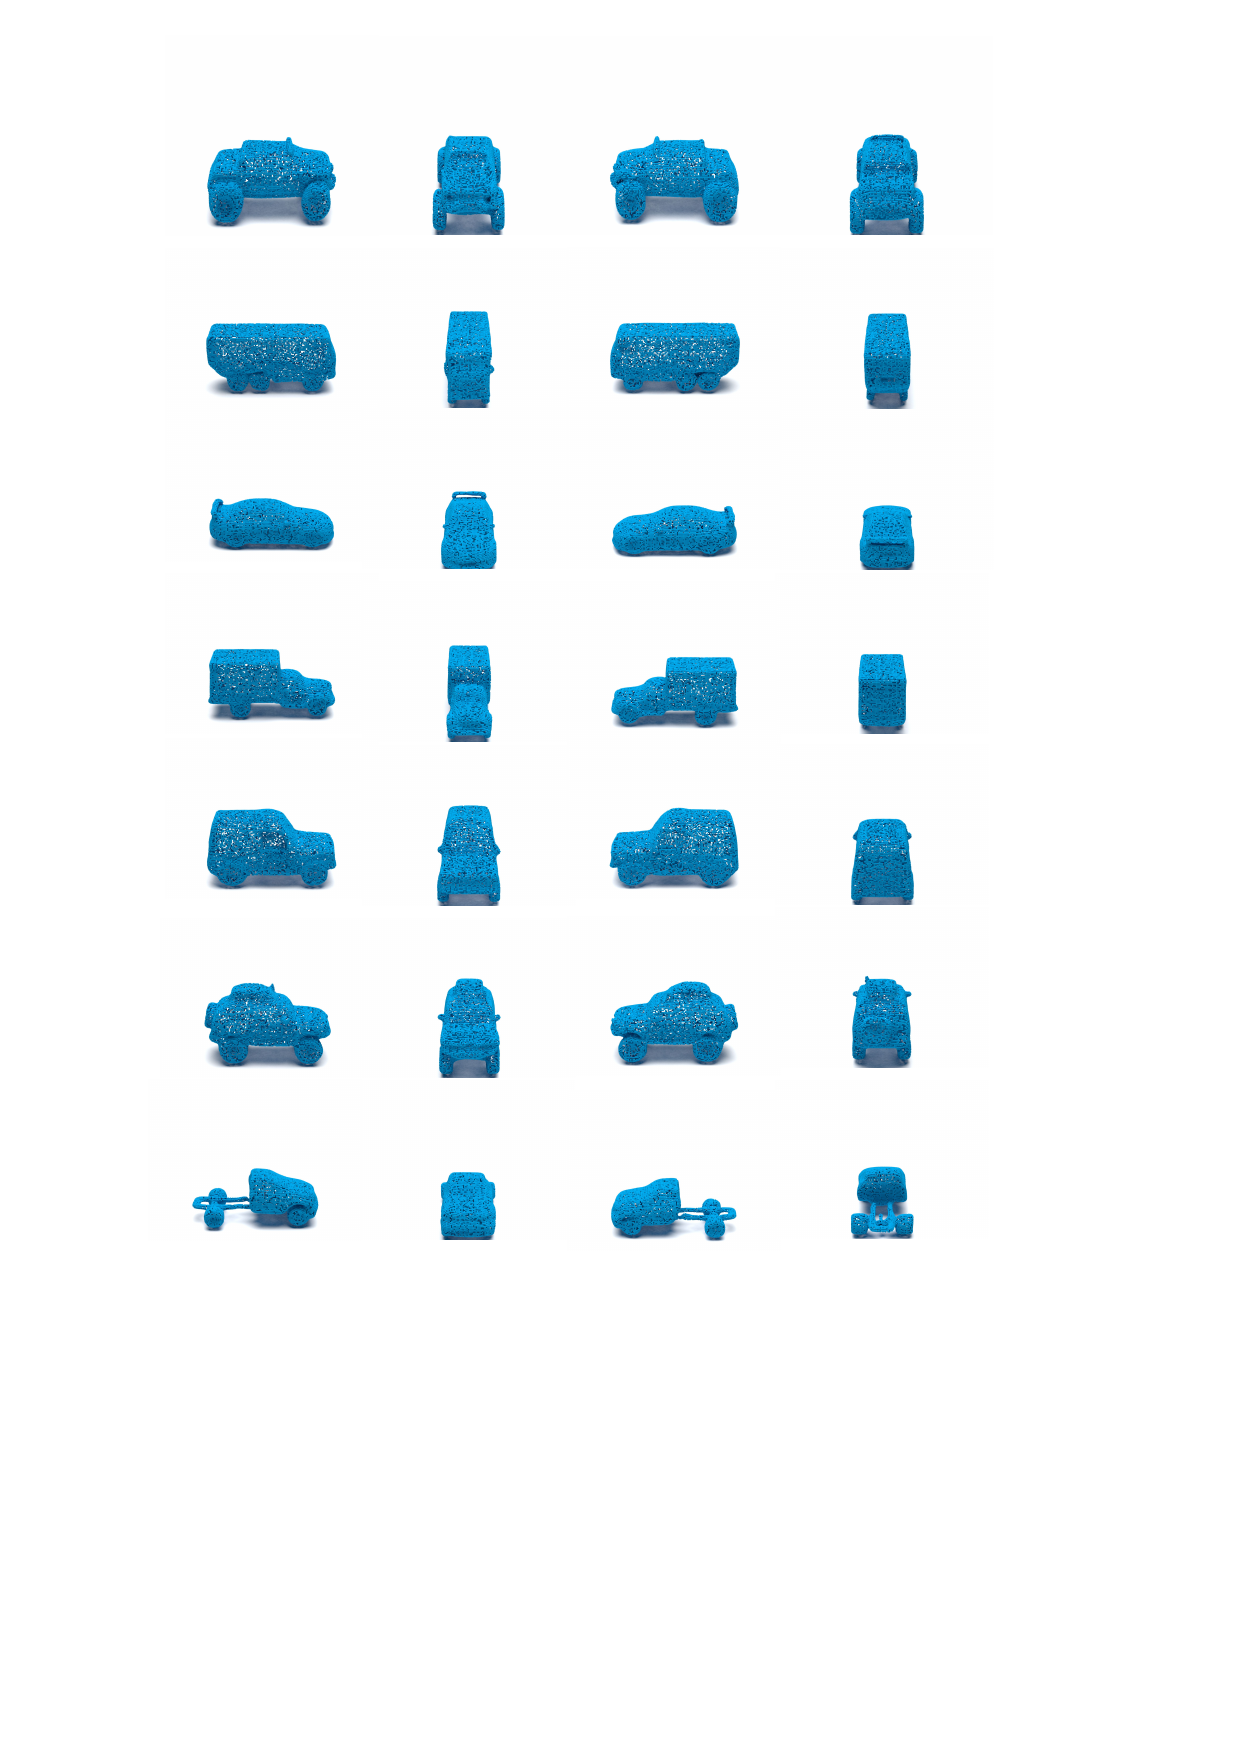}
    % \hfill\subcaptionbox*{\centering RGB}[0.19\linewidth]
    % \hfill\subcaptionbox*{\centering Depth}[0.19\linewidth]
    % \hfill\subcaptionbox*{\centering Shape}[0.19\linewidth]
    % \hfill\subcaptionbox*{\centering  RGB}[0.19\linewidth]
    % \hfill\subcaptionbox*{\centering Depth}[0.19\linewidth]
    % \hfill\subcaptionbox*{\centering Shape}[0.19\linewidth]
    % \hfill\subcaptionbox{Airplane}[0.12\linewidth]
    
  \caption{Generated cars from more angles.}
  \label{fig:car}
%   \vspace{-15pt}
\end{figure*}

\begin{figure*}[t]
  \centering
%   \fbox{\rule{0pt}{3in} \rule{0.9\linewidth}{0pt}}
  \includegraphics[width=0.8\linewidth]{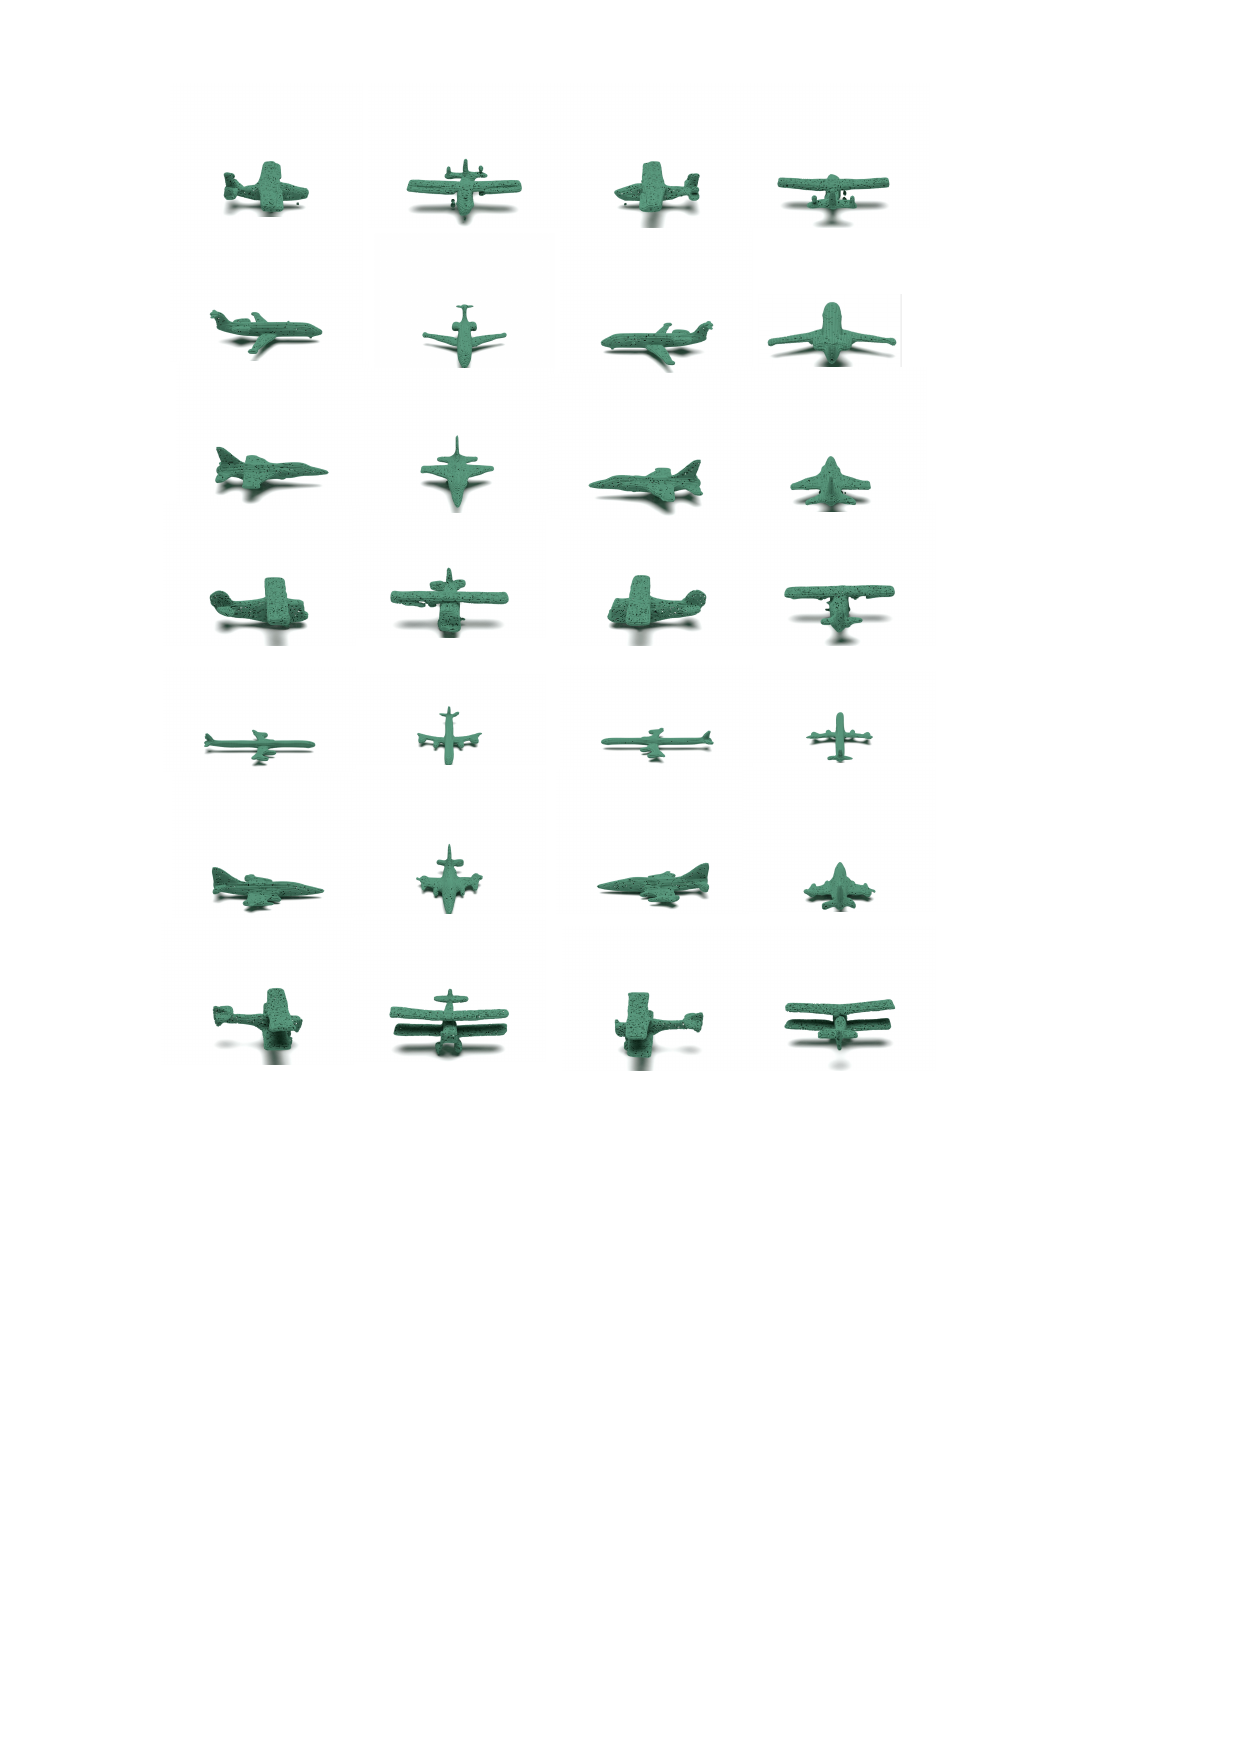}
    % \hfill\subcaptionbox*{\centering RGB}[0.19\linewidth]
    % \hfill\subcaptionbox*{\centering Depth}[0.19\linewidth]
    % \hfill\subcaptionbox*{\centering Shape}[0.19\linewidth]
    % \hfill\subcaptionbox*{\centering  RGB}[0.19\linewidth]
    % \hfill\subcaptionbox*{\centering Depth}[0.19\linewidth]
    % \hfill\subcaptionbox*{\centering Shape}[0.19\linewidth]
    % \hfill\subcaptionbox{Airplane}[0.12\linewidth]
    
  \caption{Generated airplanes from more angles.}
  \label{fig:airplane}
%   \vspace{-15pt}
\end{figure*}

% \vspace{100cm}

% To split the supplementary pages from the main paper, you can use \href{https://support.apple.com/en-ca/guide/preview/prvw11793/mac#:~:text=Delete%20a%20page%20from%20a,or%20choose%20Edit%20%3E%20Delete).}{Preview (on macOS)}, \href{https://www.adobe.com/acrobat/how-to/delete-pages-from-pdf.html#:~:text=Choose%20%E2%80%9CTools%E2%80%9D%20%3E%20%E2%80%9COrganize,or%20pages%20from%20the%20file.}{Adobe Acrobat} (on all OSs), as well as \href{https://superuser.com/questions/517986/is-it-possible-to-delete-some-pages-of-a-pdf-document}{command line tools}.
